# Supplementary material for: Assessing the SCAN functional for itinerant electron ferromagnets
Source: arXiv:1806.11289 ancillary file (2018-06-29)
Supplement: Supplementary file 1 [file SupplementaryMaterials.pdf]

# Assessing the SCAN functional for itinerant electron ferromagnets —Supplementary Material

M. Ekholm,[1,2,*] D. Gambino,[1] H. J. M. Jönsson,[1]
F. Tasnádi,[1] B. Alling,[1,3] and I. A. Abrikosov[1,2,4]

[1]*Department of Physics, Chemistry and Biology (IFM)*
*Linköping University, SE-58183 Linköping, Sweden*
[2]*Swedish e-Science Research Centre (SeRC),*
*Linköping University, SE-58183 Linköping, Sweden*
[3]*Max-Planck-Institut für Eisenforschung GmbH,*
*Max-Planck Strasse 1, 40237 Düsseldorf, Germany*
[4]*Materials Modeling and Development Laboratory, National University of Science and Technology "MISIS", 119049 Moscow, Russia*

(Dated: May 25, 2018)

*Electronic address: marekh@ifm.liu.se

**fcc-Fe**

In Fig. S1 we show total energy as a function of volume for non-magnetic fcc-Fe and ferromagnetic bcc-Fe. LSDA predicts that non-magnetic fcc-Fe is lower in energy than ferromagnetic

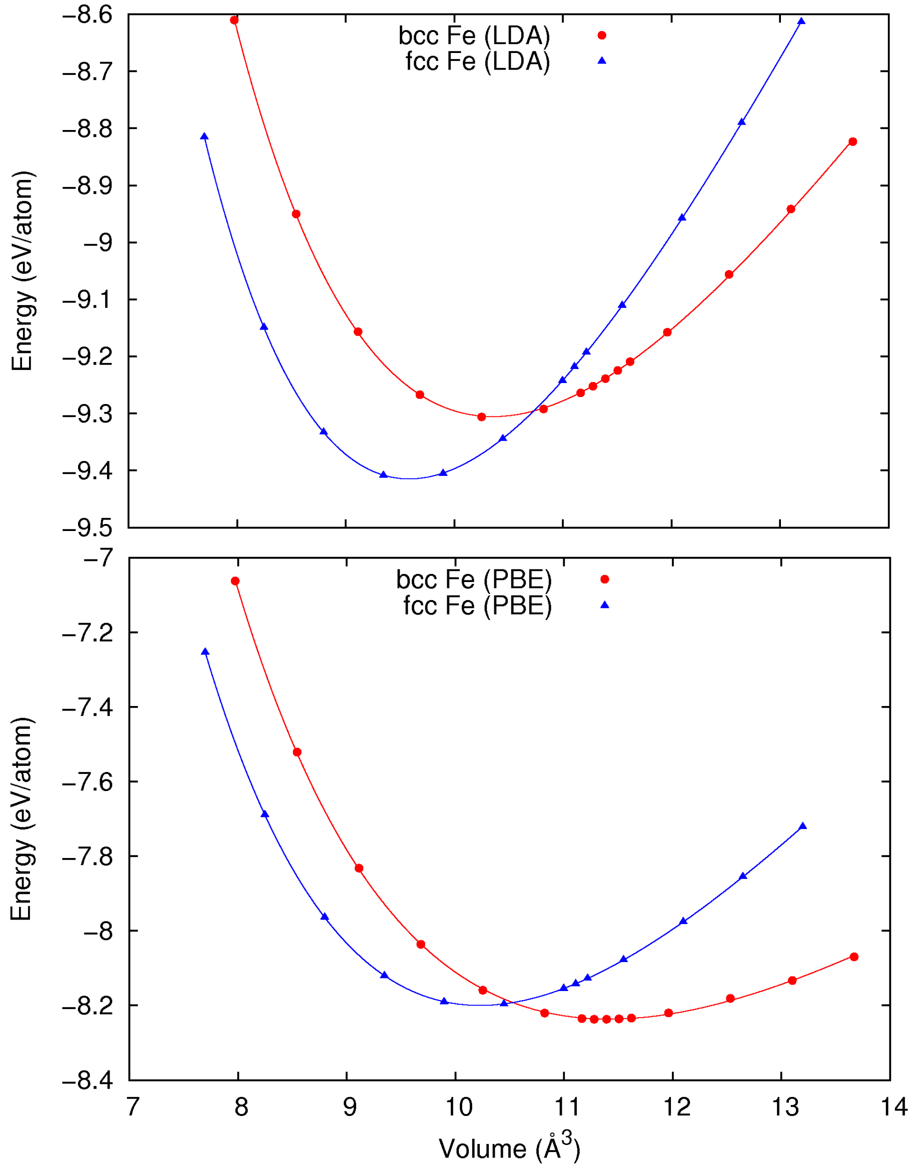


FIG. 1: Total energy calculated with the VASP code for nonmagnetic fcc-Fe and ferromagnetic bcc-Fe with the L(S)DA (top panel) (b) PBE (bottom panel) functionals.

bcc-Fe at the equilibrium volume. However, at the experimental volume of bcc-Fe (11.64 Å$^3$), the ferromagnetic bcc-solution is favoured. The PBE functional favours ferromagnetic bcc-Fe at the equilibrium volume.

### Density of states

Figs. S2–S4 show the density of states (DOS) calculated with the VASP code using the LSDA, PBE and SCAN functionals. The DOS is in each case evaluated at the equilibrium volume obtained with the respective functional.

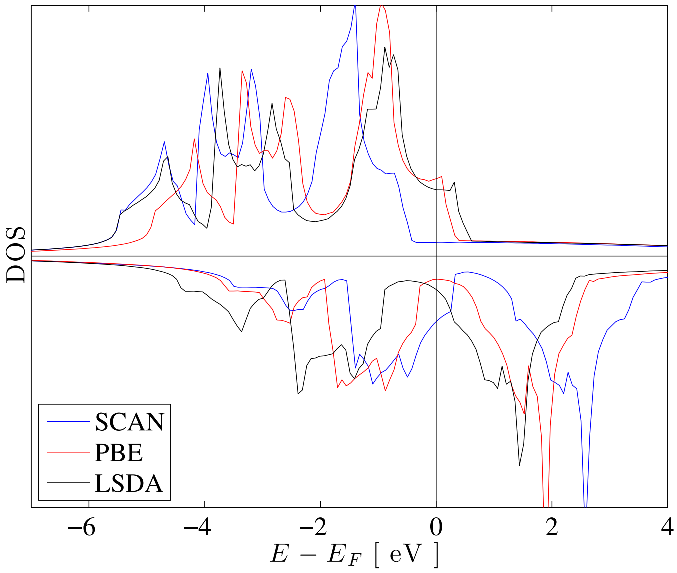


FIG. 2: (Color online) Spin-resolved DOS for bcc-Fe calculated at the experimental volume with the VASP code for the SCAN (blue), PBE (red), and LSDA (black) functionals, where $E_F$ is the Fermi energy.

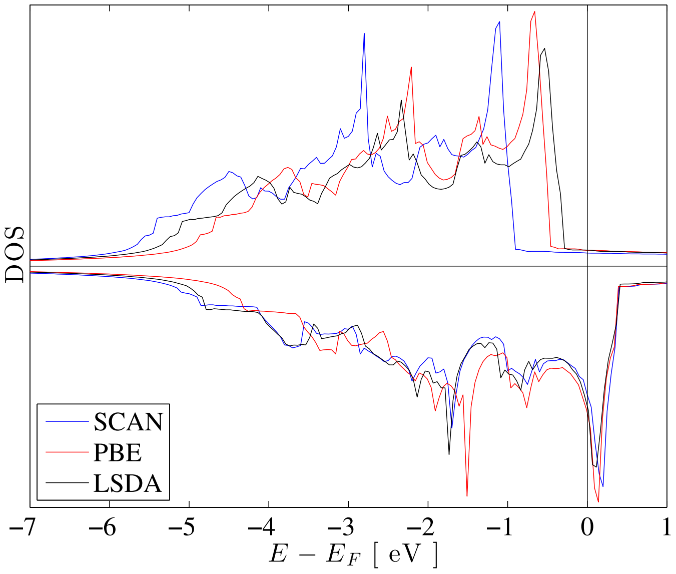


FIG. 3: (Color online) Spin-resolved DOS for fcc-Ni calculated at the experimental volume with the VASP code for the SCAN (blue), PBE (red), and LSDA (black) functionals, where $E_F$ is the Fermi energy.

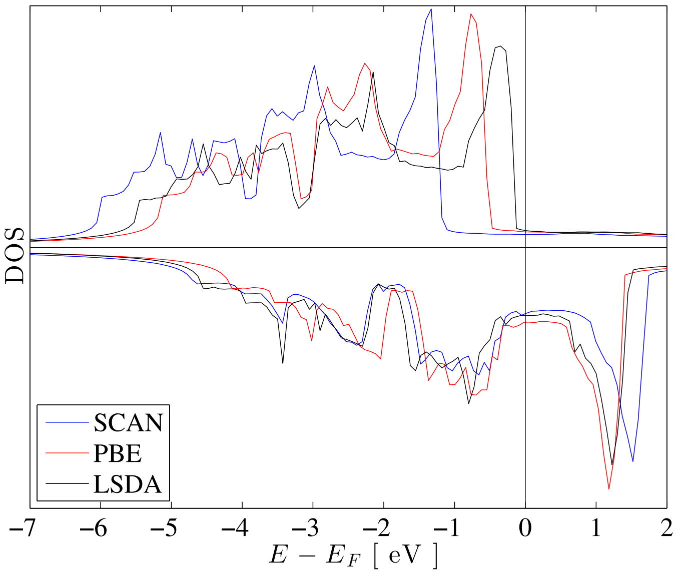


FIG. 4: (Color online) Spin-resolved DOS for hcp-Co calculated at the experimental volume with the VASP code for the SCAN (blue), PBE (red), and LSDA (black) functionals, where $E_F$ is the Fermi energy.
